# Supplementary material for: Collective conical intersections through light-matter coupling in a cavity
Source: arXiv:1806.07252 ancillary file (2018-08-09)
Supplement: Supplementary file 1 [file support.pdf]

# Collective conical intersections through light-matter coupling in a cavity

Oriol Vendrell<sup>1,\*</sup>

<sup>1</sup>*Department of Physics and Astronomy, Aarhus University, Ny Munkegade 120, 8000 Aarhus C, Denmark<sup>†</sup>*

(Dated: August 9, 2018)

## ENSEMBLE-CAVITY HAMILTONIAN IN THE SINGLE-EXCITATION SPACE

The matrix representation of

$$\hat{H}_{\text{cav-el}} = \hat{H}_{\text{el}} + \hat{H}_{\text{cav}} \quad (1)$$

in the single excitation space, where the operators are defined in the main text, is constructed in the basis of eigenstates of the non-interacting system, in which the second term in Eq. (3) of the main text is missing. The eigenstates of the non-interacting ensemble-cavity Hamiltonian are referred to as  $|1_c, 0_m\rangle$  for the excited cavity and all molecules in their ground state, and  $|0_c, \kappa_m\rangle$ , for the ground state cavity and the  $\kappa$ -th molecule singly excited. As usual the corresponding matrix elements are parameterized by the nuclear position coordinates of the molecules in the ensemble, which results in diagonal terms

$$\langle 1_c, 0_m | \hat{H}_{\text{cav-el}} | 1_c, 0_m \rangle(\mathbf{R}) = \frac{3}{2} \hbar \omega_c + \sum_{\kappa=1}^N V_0^{(\kappa)}(R_\kappa), \quad (2)$$

$$\langle 0_c, \nu_m | \hat{H}_{\text{cav-el}} | 0_c, \nu_m \rangle(\mathbf{R}) = \frac{1}{2} \hbar \omega_c + V_1^{(\nu)}(R_\nu) + \sum_{\kappa \neq \nu}^N V_0^{(\kappa)}(R_\kappa), \quad (3)$$

where  $V_j^{(\kappa)}(R_\kappa)$  is the  $j$ -th electronic state potential energy surface of the  $\kappa$ -th molecule,  $N$  is the total number of molecules and  $\omega_c$  the angular frequency of the cavity mode. The off-diagonal terms correspond to the dipole coupling of the molecules to the cavity mode

$$\langle 1_c, 0_m | \hat{H}_{\text{cav-el}} | 0_c, \nu_m \rangle(\mathbf{R}) = g \vec{\epsilon}_c \cdot \vec{\mu}_{01}^{(\nu)}(R_\nu), \quad (4)$$

where  $\vec{\mu}_{01}^{(\nu)}$  is the transition dipole matrix element among ground and first excited electronic states of the  $\nu$ -th molecule,  $\vec{\epsilon}_c$  is the polarization direction of the cavity mode and  $g$  is the coupling factor defined in the main text. In Eq. (4), the non-energy conserving terms arising from  $\vec{D}(\hat{a}^\dagger + \hat{a})$  in the main Eq. (3) are not present because they couple states outside the single excitation space, for example the absolute ground state and doubly excited states  $|0_c, 0_m\rangle$  and  $|1_c, \kappa_m\rangle$ , respectively. This is the rotating wave approximation and results in the well known Tavis-Cummings model for an ensemble of two-state atoms [1], now parameterized by the internal coordinates of each molecule in the ensemble.

Subtracting from the diagonal terms the total ground state energy

$$\langle 0_c, 0_m | \hat{H}_{\text{cav-el}} | 0_c, 0_m \rangle(\mathbf{R}) = \frac{1}{2} \hbar \omega_c + \sum_{\kappa=1}^N V_0^{(\kappa)}(R_\kappa) \quad (5)$$

yields a compact representation of the single excitation Hamiltonian matrix

$$\mathcal{H}_{\text{el-cav}}^{[1]}(\mathbf{R}) = \begin{pmatrix} \hbar \omega_c & \gamma^{(1)}(R_1) & \gamma^{(2)}(R_2) & \gamma^{(3)}(R_3) & \cdots \\ \gamma^{(1)}(R_1) & \Delta^{(1)}(R_1) & 0 & 0 & \cdots \\ \gamma^{(2)}(R_2) & 0 & \Delta^{(2)}(R_2) & 0 & \cdots \\ \gamma^{(3)}(R_3) & 0 & 0 & \Delta^{(3)}(R_3) & \cdots \\ \vdots & \vdots & \vdots & \vdots & \ddots \end{pmatrix}, \quad (6)$$

which is Eq. (4) in the main text.

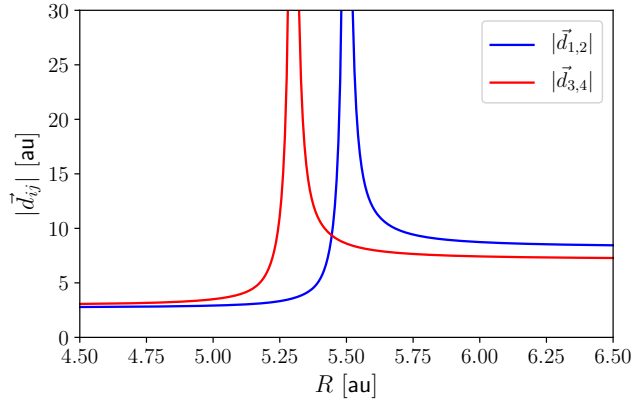

FIG. 1. Absolute value of the non-adiabatic coupling vector  $|\langle\psi_i|\vec{\nabla}_R|\psi_j\rangle|$  between crossing pairs of polaritonic states along the same potential energy surface cut of Fig. 1c.

### NON-ADIABATIC COUPLINGS BETWEEN POLARITONIC STATES

As expected, the non-adiabatic coupling (NAC) vector at a CCI diverges to infinity in the same way as for its intra-molecular counterparts, which is seen in Fig. (1). There, the absolute value of the NAC vector  $|\langle\psi_i|\vec{\nabla}_R|\psi_j\rangle|$  computed numerically is plotted for various pairs of electronic states along the same geometrical cut of Fig. (??c), and the divergence to infinity at the points of CCI is clearly appreciated.

---

\* e-mail: [oriol.vendrell@pci.uni-heidelberg.de](mailto:oriol.vendrell@pci.uni-heidelberg.de)

† Current affiliation: Theoretische Chemie, Physikalisch-Chemisches Institut, Universität Heidelberg, INF 229, 69120 Heidelberg, Germany

[1] M. Tavis and F. Cummings, *Phys. Lett. A* **25**, 714 (1967).
